# Supplementary material for: The State of Robot Motion Generation
Source: arXiv:2410.12172 source file (2024-12-16)
Supplement: Supplementary file 1 [file appendix.tex]

\section*{Appendices}

\section{(Partially Observable) Markov Decision Processes}
\label{sec:pomdp}

A {\bf Markov Decision Processes (MDP)} is a framework for optimizing agent behavior in sequential decision-making problems. An MDP consists of a set of states $S$, set of actions $A$, transition probabilities between states $T(s_{t+1} \mid s_t, a_t)$, and a reward function $R(s_t,a_t,s_{t+1})$. Temporally discretizing when the agent must act simplifies the structure and use of the corresponding policies. Additionally, the reward function $R(s_t,a_t,s_{t+1})$ provides a flexible way to specify desired behaviors. MDPs assume the Markov property as defined in the transition function $T(s_{t+1} \mid s_t, a_t)$, which states that the next state $s_{t+1}$ is dependent only on the previous state $s_t$. MDPs assume full observability of the state. 

A {\bf Partially Observable Markov Decision Process (POMDP)} consists of a set of states $S$, set of actions $A$, transition probabilities between states $T(s_{t+1} \mid s_t, a_t)$, a reward function $R(s_t,a_t,s_{t+1})$, a set of observations $O$, and an observation function $O(o_t|s_t,a_{t-1})$. POMDPs do not assume full observability of the state and instead receive observations $o$, which can be used in conjunction with the observation model $O(o_t|s_t,a_{t-1})$ to compute the belief state. The belief state acts as a distribution over true underlying states and can be computationally challenging to accurately represent for most real-world robotics problems. 

\section{Low-level Controllers}
\label{sec:pid}

{\bf Proportional-integral-derivative (PID)} controllers output controls based on an \textit{error value} $e(t)$ that measures the difference between a desired value of a tracked quantity and the actual value \cite{astromFeedbackSystemsIntroduction2008}. This controller is a weighted sum of three primary components:
\begin{itemize}
    \item \textbf{Proportional}: a term proportional to $e(t)$;
    \item \textbf{Integral}: a term that accounts for the past values of $e(t)$ by integrating over $e(t)$ over time;
    \item \textbf{Derivative}: a term that accounts for the future values of $e(t)$ by using the current rate of change of $e(t)$.
\end{itemize}

For a viable PID controller, the weights associated with these terms have to be tuned. Depending on the use case, these weights can be set to zero, resulting in PD and PI controllers. These controllers are simple to implement, are robust if properly tuned, and can run on simple micro-controllers. Hence, these controllers are heavily employed for industrial applications and low-level actuation control for robotic applications.  

At the same time, PID controllers exhibit limitations when applied to nonlinear systems and do not easily incorporate predictive control. PID controllers target short-horizon goals and consequently, they struggle with long-horizon tasks. These limitations hinder their suitability for deployment in high-level, complex tasks requiring longer-horizon planning. Furthermore, they require manual tuning for each system, which complicates their deployment across a wide array of systems.

\section{Path Tracking Controllers}
\label{sec:path_tracking}

{\bf Pure-Pursuit controller} \cite{PurePursuit1991} is an example path tracking controller, which aims to reduce the heading error of a vehicle along a path that is treated as a series of waypoints. It chooses a point on the path at a certain distance ahead of the robot's position as the look-ahead point. The controller then calculates a steering angle using a geometric model to navigate to this look-ahead point. This controller is simple to implement and can track smooth or moderately curved paths well. Due to its purely geometric model, however, performance can degrade for heavily curved paths or sharp turns. 

The {\bf Stanley controller} \cite{Stanley2006} can also deal with dynamics and aims to perform trajectory following. It minimizes a lateral cross-track error (the perpendicular distance from the vehicle to the path) and the heading error. It also accounts for robot velocity to compute the steering angle. The Stanley controller can address a variety of conditions, including varying speeds and complex paths but can still struggle with sharp turns at high velocities.

For robotic arms, the simplest tracking controllers are decentralized PID-based approaches where there is a separate controller for each joint. They can perform poorly, however, under non-linear dynamics, which has motivated the development of more sophisticated alternatives. For instance,  Computed Torque Control (CTC) \cite{CTC} leverages the dynamic model of the robot. It calculates the necessary torques to achieve a desired trajectory while compensating for the robot's dynamics, such as inertia, Coriolis, and centrifugal forces. Alternatively, Sliding Mode Control (SMC) \cite{SMC}  forces the system states to follow a desired trajectory by driving them to a predefined sliding surface. The surface is typically chosen such that when the system states are on this surface, the system behaves according to the desired dynamics. 

%Computed torque control (CTC) combined with PID and sliding mode control (SMC)  are some more sophisticated solutions. Adaptive methods have also been popular to estimate unknown parameters. Fuzzy Logic \cite{de1995applications} and neural-network-based approaches \cite{PIDNN} \cite{hu2006fuzzy} have been popular for estimation and control. Fractional Order PID (FOPID) control extends the traditional PID controller by incorporating fractional calculus into the integral and derivative components, resulting in more flexible control dynamics. This was used to further develop a Fractional Order Fuzzy PID controller for trajectory tracking \cite{mohammed2016trajectory}. Perfect modeling of the system is an impossible task. However, purely robust techniques rely on an exact model. Therefore, a feasible solution is to develop robust and adaptive methods \cite{ajwad2015systematic}.

\section{(Deep) Reinforcement Learning Basics}
\label{sec:rl_basics}

Reinforcement Learning (RL) is a method for autonomously acquiring a desired policy $\pi$ for sequential decision making tasks. RL traditionally operates over a (PO)MDP (see Appendix \ref{sec:pomdp}). The key components of RL include the agent, environment, states $s_t$, actions $a_t$, rewards $R(s_t,a_t)$, policy $\pi$, a value function $V(s_t)$, and a Q-function $Q(s_t,a_t)$. The agent starts with an initial policy, which could be random or based on some heuristic. During interaction, the agent observes the current state $s_t$, selects an action $s_t$ based on the current policy $\pi$, executes the action in the environment, and receives a reward $R(s_t, a_t)$ while the environment transitions to a new state. The agent updates its policy and/or value functions based on the reward and the new state, aiming to improve the policy to {\bf maximize the expected cumulative reward} $J(\pi)$ as expressed by the following function (where $\gamma < 1$ is a discounting factor):

\vspace{-.1in}
\begin{equation}
J(\pi) = \mathbb{E}_{\tau \sim \pi} \left[ \sum_{t=0}^{\infty} \gamma^t R(s_t, a_t) \right]
\label{eq:rl_objective}
\end{equation}

RL does not need a proper model of the environment as a prerequisite as it can learn a model only from experience. This experience does not require the RL algorithms to explicitly interact with the environment. Instead it is possible to learn policies that maximize Eq.\ref{eq:rl_objective} given only offline state transition data. 

Several algorithms embody these principles, including Q-learning, SARSA, and Policy Gradient methods. {\bf SARSA} is an on-policy algorithm that updates Q-values based on the actual actions taken, adjusting the Q-value for the current state-action pair using the reward and the Q-value of the next state-action pair:
$$Q(s_t,a_t) \leftarrow Q(s_t,a_t) + \alpha [r + \gamma Q(s_{t+1},a_{t+1}) - Q(s_t,a_t)]$$
where $\alpha$ is the learning rate and $\gamma$ is the discount factor. 

{\bf Q-learning} is an off-policy algorithm where the agent learns the Q-function directly, updating Q-values using the Bellman equation:
$$Q(s_t, a_t) \leftarrow Q(s_t,a_t) + \alpha [r + \gamma \cdot max_{a_{t+1}}Q(s_{t+1}, a_{t+1}) - Q(s_t, a_t)]$$

{\bf Policy Gradient methods} directly adjust the policy parameters to maximize expected rewards using gradient decent. Through repeated interactions, updates, and learning, the agent aims to refine its policy to achieve optimal behavior, effectively navigating the environment to accomplish its goals.

RL has to {\bf  balance exploitation and exploration} where it either refines the currently high valued behaviors further or explores other options that could be advantageous. Exploitation by repeating known valuable behaviors does not only refine small inefficiencies and explores high reward regions, but also learns the expectation of discounted future rewards over all forms of uncertainty so that the policy can find the most robust behaviors.  RL has seen superhuman performance at games such as alpha go \cite{go}, DotA and Atari games \cite{atari}. 

{\bf Deep RL (DRL):} RL was initially limited to discrete actions and state spaces with methods, such as tabular Q learning, where a table of Q values is stored for each discrete state and action pair. Robotics operates over continuous spaces and it becomes intractable to maintain such a table as dimensionality increases. For RL to operate in continuous spaces, similar states need to be matched to build the expectation of discounted future rewards for each state. To manually obtain a useful metric of similarity between states is difficult and is heavily dependent on the numerical description of the state. Furthermore, storing this information and accessing it in a reasonable time upon inference is a challenge. This motivated the application of deep neural networks (DNNs) to RL. DNNs facilitate the calculation of the expectation as DNNs can autonomously match similar continuous states through smooth interpolation in feature space. DNNs compactly store data and can be queried quickly and inexpensively. 

%The uniqueness and usefulness of RL comes from a variety of its attributes. These attributes include an inexpensive online runtime, only needing data, maximizing expectation, the ability to leverage domain randomization, and closed-loop control. The inexpensive runtime of RL is because the resultant policy of a RL agent is generally in the form of a MLP which can be queried at the low cost of a few matrix multiplications and activation function calls.  RL follows the objective of maximizing the expectation of discounted future rewards at each step over uncertainty and randomness which is a critical advantage of DRL as this develops robust behaviors. The crucial elements that enable this is the repeating rollouts from the start position and the ability of DNNs to autonomously match similar states and compound the information over instances. 

%Adjacent to this is the reactive nature of DRL as it utilizes closed-loop control. The training distribution specifically covers the areas that the randomness of state transitions leads to which allows DRL policies to handle randomness in a reactive manner which provides additional robustness in addition to finding the highest expected value trajectory [not sure if I need to cite this]. 

\vspace{-.1in}
